# Supplementary material for: Towards mitigating uncann(eye)ness in face swaps via gaze-centric loss terms
Source: arXiv:2402.03188 source file (2024-02-05)
Supplement: Supplementary file 1 [file appendix.tex]

\appendix
\section{}

All face swaps were generated using a NVIDIA GeForce RTX 2080 Super.  The exact run configurations used to generate our face swaps are outlaid.  For training parameters, refer to Figure~\ref{fig:train_params}.  For merge parameters, refer to Table~\ref{tab:merge_params}.

\begin{figure}[th!]
    \centering
    \includegraphics[width=1\linewidth]{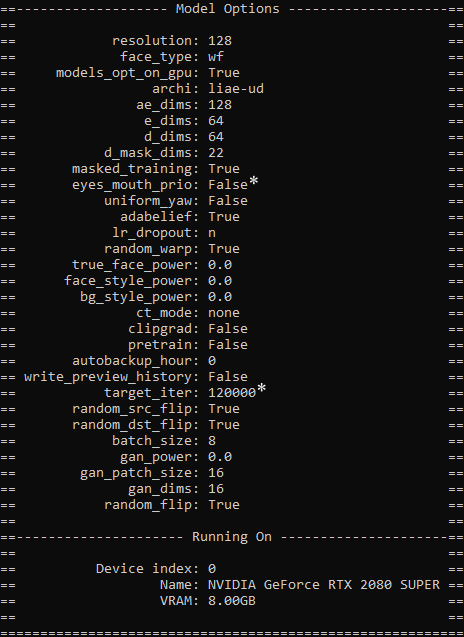}
    \caption{Training parameters used to when generating all face swap stimuli.  Note that the LIAE architecture is classified as a SAEHD model in DFL's configurations.  The \textbf{eyes\_mouth\_prio} parameter was set to true when the proposed gaze term was disabled.  \textbf{target\_iter} varied depending on training phase (100k iterations pretraining, 20k iterations on the end pair of identities).}
    \label{fig:train_params}
\end{figure}

\begin{table}
\centering
\begin{tabular}{|l|c|}
\hline
\textbf{Parameter}                     & \textbf{Value}              \\ \hline
mode                                   & (1) overlay                 \\ \hline
mask mode                              & (4) learned-prd*learned-dst \\ \hline
erode mask modifier                    & 20                          \\ \hline
blur mask modifier                     & 80                          \\ \hline
motion blur power                      & 0                           \\ \hline
output face scale modifier             & 0                           \\ \hline
color transfer to predicted face       & rct                         \\ \hline
sharpen mode                           & (0) None                    \\ \hline
super resolution power                 & 0                           \\ \hline
image degrade by denoise power         & 0                           \\ \hline
image degrade by bicubic rescale power & 0                           \\ \hline
degrade color power of final image     & 0                           \\ \hline
number of workers                      & 12                          \\ \hline
\end{tabular}

\caption{Merge parameters used to generate our face swap stimuli after training.  Note that the original video clips were 1920x1080 pixels at 24 frames per second and faces were extracted at 512x512 pixels.}
\label{tab:merge_params}
\end{table}
